# Supplementary material for: The extremal length systole of the cube punctured at its vertices
Source: arXiv:2404.00336 ancillary file (2026-07-15)
Supplement: Supplementary file 1 [file integrals.pdf]

```
In [1]: # This file provides rigorous estimates for elliptic integrals appearing in
        # the paper
        # "The extremal length systole of the cube punctured at its vertices" by Sa
        # muel Dobchies
        # and Maxime Fortier Bourque

        # Functions to compute complete elliptic integrals of the first kind and th
        # eir ratios

        def complementary_modulus(k):
            return sqrt(1-k^2)

        def ellipticK(k):
            return pi/2/CBF(complementary_modulus(k)).agm1()

        def ellipticKprime(k):
            return pi/2/CBF(k).agm1()

        def KoverKprime(k):
            return ellipticK(k)/ellipticKprime(k)
```

```
In [2]: # Face curves

        a = (sqrt(3)+1)/sqrt(2)

        8*KoverKprime(1/a^4)
```

```
Out[2]: [3.12680384539222 +/- 8.07e-15]
```

```
In [3]: # Diagonal curves

        t = 2*a^4/(1+a^4)

        4*KoverKprime(1/sqrt(t))
```

```
Out[3]: [4.1335929781133 +/- 2.81e-14]
```

```
In [4]: # Staple curves

        t = 1+1/a^4

        4*KoverKprime(1/sqrt(t))
```

```
Out[4]: [6.9282032302755 +/- 2.74e-14]
```

```
In [5]: # Hexagon curves

        6*KoverKprime(1/3)
```

```
Out[5]: [3.83778471351302 +/- 9.40e-15]
```

In [6]: *#Tripod curves*

```
6*KoverKprime(2*sqrt(2)/3)
```

Out[6]: [9.3804115361767 +/- 5.12e-14]

In [7]: *# Some constants used in the cells below*

*# RBF stands for "real ball field", which uses interval arithmetic*

```
B = RBF(5-2*sqrt(6))
```

```
C = RBF(5+2*sqrt(6))
```

In [8]: *# Lower bound on  $r_{\theta}$*

```
r1 = QQ(-9.0795)
```

```
eps = QQ(1/10^12)
```

*# A Lower bound on  $I_{\{r1\}}(r1, \theta)$*

```
I1 = RBF(CBF.integral(lambda x, _: sqrt(abs((x-r1)/(x*(x-B)*(x-C)*(x^2+(2/3)*x+1))))),r1+eps,-eps))
```

*# An upper bound on  $I_{\{r1\}}(B, C)$*

```
I2 = RBF(CBF.integral(lambda x, _: sqrt(abs((x-r1)/(x*(x-B)*(x-C)*(x^2+(2/3)*x+1))))),B+eps,C-eps))
```

```
I2 += 2*sqrt(eps*(B+eps-r1)/(B*(C-B-eps)*(B^2+(2/3)*B+1)))
```

```
I2 += 2*sqrt(eps*(C-r1)/((C-eps)*(C-eps-B)*((C-eps)^2+(2/3)*(C-eps)+1)))
```

```
delta = I1-I2
```

```
print('delta is bounded below by',delta.lower(),'at r1=',RDF(r1))
```

delta is bounded below by 2.64430399971038e-6 at r1= -9.0795

In [9]: *# Upper bound on  $r_{\theta}$*

```
r2 = QQ(-9.0791)
```

```
eps = QQ(1/10^12)
```

```
# An upper bound on  $I_{\{r2\}}(r2, \theta)$ 
```

```
I1 = RBF(CBF.integral(lambda x, _: sqrt(abs((x-r2)/(x*(x-B)*(x-C)*(x^2+(2/3)*x+1))))),r2+eps,-eps))
```

```
I1 += (3/2)*eps*sqrt(eps/(-(r2+eps)*(B-r2-eps)*(C-r2-eps)*((r2+eps)^2+(2/3)*(r2+eps)+1))))
```

```
I1 += RBF(2*sqrt(-eps*r2))
```

```
# A Lower bound on  $I_{\{r2\}}(B, C)$ 
```

```
I2 = RBF(CBF.integral(lambda x, _: sqrt(abs((x-r2)/(x*(x-B)*(x-C)*(x^2+(2/3)*x+1))))),B+eps,C-eps))
```

```
delta = I1-I2
```

```
print('delta is bounded above by',delta.lower(),'at r2=',RDF(r2))
```

delta is bounded above by -2.42550805931719e-6 at r2= -9.0791

```

In [10]: # Upper bound on the extremal length of beta

r = QQ(-9.0792887)

eps = QQ(1/10^12)

# Upper bound on the numerator

# First bound the integral itself
num = RBF(CBF.integral(lambda x, _: sqrt(abs((x-r)/(x*(x-B)*(x-C)*(x^2+(2/3)*x+1))))),eps,B-eps))
num += 2*sqrt(eps*(eps-r)/((B-eps)*(C-eps)))
num += 2*sqrt(eps*(B-r)/((B-eps)*(C-B)*((B-eps)^2+(2/3)*(B-eps)+1)))
# Then multiply by 2
num = 2*num

# Lower bounds on the two terms on the denominator

I1 = RBF(CBF.integral(lambda x, _: sqrt(abs((x-r)/(x*(x-B)*(x-C)*(x^2+(2/3)*x+1))))),r+eps,-eps))

I2 = RBF(CBF.integral(lambda x, _: sqrt(abs((x-r)/(x*(x-B)*(x-C)*(x^2+(2/3)*x+1))))),B+eps,C-eps))

denom = min(I1,I2)

# Upper bound on the ratio

E_up = num/denom

print('The extremal length of beta is bounded above by',E_up.upper())

```

The extremal length of beta is bounded above by 1.42159304798927

In [11]: *# Lower bound on the extremal length of beta*

```
r = QQ(-9.0792887)

eps = QQ(1/10^12)

# Lower bound on the numerator

num = 4*RBF(CBF.integral(lambda x, _: sqrt(abs((x-r)/(x*(x-B)*(x-C)*(x^2
+(2/3)*x+1))))),eps,B-eps))

# Upper bound on the denominator

# For this, we need both lower and upper bounds on I_r(r,θ) and I_r(B,C)

I1_low = RBF(CBF.integral(lambda x, _: sqrt(abs((x-r)/(x*(x-B)*(x-C)*(x^2
+(2/3)*x+1))))),r+eps,-eps))

I2_low = RBF(CBF.integral(lambda x, _: sqrt(abs((x-r)/(x*(x-B)*(x-C)*(x^2
+(2/3)*x+1))))),B+eps,C-eps))

I1_up = I1_low + (3/2)*eps*sqrt(eps/(-(r+eps)*(B-r-eps)*(C-r-eps)*((r+eps)^
2+(2/3)*(r+eps)+1))) + RBF(2*sqrt(-eps*r))

I2_up = I2_low + 2*sqrt(eps*(B+eps-r)/(B*(C-B-eps)*(B^2+(2/3)*B+1)))+ 2*sqrt
(eps*(C-r)/((C-eps)*(C-eps-B)*((C-eps)^2+(2/3)*(C-eps)+1)))

I1 = RBF(RIF(I1_low.lower(),I1_up.upper()))
I2 = RBF(RIF(I2_low.lower(),I2_up.upper()))

# We also need an upper bound on J_r(C,r) which we obtain after the change
of variable in the paper

J1 = RBF(CBF.integral(lambda y, _: sqrt(abs((y-1/r)/((y-B)*(y-C)*(y^2+(2/
3)*y+1))))),1/r+eps,B-eps))
J1 += (3/2)*eps*sqrt(eps/((B-1/r-eps)*(C-1/r-eps)*((1/r)^2+(2/3)/r+1)))
J1 += 2*sqrt(eps*(B-1/r)/((C-B)*((B-eps)^2+(2/3)*(B-eps)+1)))
J1 = RBF(sqrt(-r))*J1

denom = I1+I2+(4*J1/num)*abs(I1-I2)

# Lower bound on the ratio

E_low = num/denom

print('The extremal length of beta is bounded below by',E_low.lower())
```

The extremal length of beta is bounded below by 1.42158512329292

In [12]: **print**('The extremal length of an edge curve on the cube punctured at its vertices is between',(2\*E\_low).lower(),'and',(2\*E\_up).upper())

The extremal length of an edge curve on the cube punctured at its vertices is between 2.84317024658584 and 2.84318609597853

In [13]: *# Lower bound on the extremal length of double-edge curves*

```
(8/(E_up)).lower()
```

Out[13]: 5.62748953458581

In [14]: *# Upper bound on the extremal length of diamond curves*

```
t = 8*a^3/((a^2+2*a)^2-(sqrt(2)-1)^2)
```

```
F = RBF(2*KoverKprime(1/sqrt(t)))
```

```
F.upper()
```

Out[14]: 5.53564498781518

In [15]: *# Lower bound on the extremal length of triangle curves*

```
(16/RBF(5.535645)).lower()
```

Out[15]: 2.89035875674830
